# Supplementary material for: From Imitation to Refinement -- Residual RL for Precise Assembly
Source: arXiv:2407.16677 source file (2024-12-12)
Supplement: Supplementary file 2 [file main_appendix.tex]

\documentclass{article}


% \usepackage{corl_2024} % Use this for the initial submission.
\usepackage[final]{corl_2024} % Uncomment for the camera-ready ``final'' version.
% \usepackage[preprint]{corl_2024} % Uncomment for pre-prints (e.g., arxiv); This is like ``final'', but will remove the CORL footnote.

\usepackage{booktabs}
\usepackage{multirow}

% The following packages can be found at http:\\www.ctan.org
\usepackage{graphicx}
\usepackage{amsmath} % assumes amsmath package installed
\usepackage{amssymb}  % assumes amsmath package installed
% \usepackage{cite}

% \usepackage[bookmarks=true,colorlinks=true,citecolor=magenta,linkcolor=cyan]{hyperref}
% \usepackage[ruled,vlined]{algorithm2e}

\usepackage{booktabs} % For formal tables
\usepackage{makecell}
\usepackage{pifont}
\usepackage{float}
\usepackage{subcaption}
\usepackage{array}
\usepackage{siunitx}
\usepackage{enumitem}
\usepackage{arydshln}
\usepackage{wrapfig}
\usepackage{caption}




\newcommand{\xmark}{\ding{55}}


% \renewcommand{\algorithmautorefname}{Algorithm}
\renewcommand{\subsectionautorefname}{Sec.}
\renewcommand{\subsubsectionautorefname}{Sec.}
\renewcommand{\figureautorefname}{Fig.}
\renewcommand{\tableautorefname}{Tab.}

\usepackage{ifthen}
\newboolean{draft-mode}
\setboolean{draft-mode}{true}
% \setboolean{draft-mode}{false}

\newcommand{\anthony}[1]{\ifthenelse{\boolean{draft-mode}}{\textcolor{magenta}{Anthony: #1}}{}}
\newcommand{\pulkit}[1]{\ifthenelse{\boolean{draft-mode}}{\textcolor{red}{Pulkit: #1}}{}}
\newcommand{\lars}[1]{\ifthenelse{\boolean{draft-mode}}{\textcolor{blue}{Lars: #1}}{}}
\newcommand{\idan}[1]{\ifthenelse{\boolean{draft-mode}}{\textcolor{green}{Idan: #1}}{}}

% \DeclareRobustCommand{\asnote}[1]{\ifthenelse{\boolean{draft-mode}}{\textcolor{cyan}{\textbf{Anthony:} #1}}{}}
% \DeclareRobustCommand{\pulkit}[1]{\ifthenelse{\boolean{draft-mode}}{\textcolor{orange}{\textbf{Pulkit:} #1}}{}}

% Commands for suggestions

% \newcommand{\pulkit}[1]{{\color{red}[Pulkit: #1]}}
% \newcommand{\anthony}[1]{{\color{magenta}[Anthony: #1]}}
% \newcommand{\lars}[1]{{\color{blue}[Lars: #1]}}
% \newcommand{\idan}[1]{{\color{green}[Idan: #1]}}


\newcommand{\methodname}{\texttt{ResiP}}
\newcommand{\lamp}{\texttt{lamp}}
\newcommand{\oneleg}{\texttt{one\_leg}}
\newcommand{\squaretable}{\texttt{square\_table}}
\newcommand{\roundtable}{\texttt{round\_table}}
\newcommand{\obschunk}{\mathbf{o_t}}
\newcommand{\statechunk}{\mathbf{s_t}}
\newcommand{\actchunk}{\mathbf{a_t}}

\newcommand{\SE}[1]{\text{SE}(#1)}
\newcommand{\SO}[1]{\text{SO}(#1)}
\newcommand{\sethree}{$\text{SE}(3)$}
\newcommand{\setwo}{$\text{SE}(2)$}
\newcommand{\sothree}{$\text{SO}(3)$}
\newcommand{\xform}{\mathbf{T}}

\newcommand{\myparagraph}[1]{\vspace{-3pt}\paragraph{#1}}
\newcommand{\myitem}{\vspace{-1.5pt}\item}

% \title{\textit{Screw Like You Mean It!} Robust Real-World Assembly from Vision with RL}
% \title{\textit{Assembly} Residual Policies for Learning Precise Corrections} 
% \title{\textit{From Imitation to Refinement} -- Residual Policy Corrections for Precise Visual Assembly}
\title{\textit{From Imitation to Refinement} -- \\Residual RL for Precise Visual Assembly\\\textit{Supplementary Materials}}
% \title{Beyond Human Demonstrations - Leveraging Residual Policies for Precise Assembly} 

% From Imitation to Refinement - Leveraging Residual Policies for Precise Assembly

% The \author macro works with any number of authors. There are two
% commands used to separate the names and addresses of multiple
% authors: \And and \AND.
%
% Using \And between authors leaves it to LaTeX to determine where to
% break the lines. Using \AND forces a line break at that point. So,
% if LaTeX puts 3 of 4 authors names on the first line, and the last
% on the second line, try using \AND instead of \And before the third
% author name.

% NOTE: authors will be visible only in the camera-ready and preprint versions (i.e., when using the option 'final' or 'preprint'). 
% 	For the initial submission the authors will be anonymized.

\author{}


\begin{document}
\maketitle

\input{appendix}

\clearpage

\bibliography{references}  % .bib

\end{document}
